# Supplementary material for: A novel in vitro device to deliver induced electromagnetic fields to cell and tissue cultures
Source: arXiv:2011.09698 ancillary file (2020-11-19)
Supplement: Supplementary file 1 [file Supporting_Material.pdf]

# Supporting Material

## ‘A novel *in vitro* device to deliver induced electromagnetic fields to cell and tissue cultures’

Rea Ravin[1,2*], Teddy X. Cai[2*], Randall H. Pursley[3], Marcial Garmendia-Cedillos[3], Tom Pohida[3], Raisa Z. Freidlin[3], Herui Wang[4], Zhengping Zhuang[4], Amber J. Giles[4], Nathan H. Williamson[2,5], Mark R. Gilbert[4], and Peter J. Basser[*2]

[*]Indicates equal contribution
[1]Celoptics, Inc., Rockville, MD, USA
[2]Section on Quantitative Imaging and Tissue Sciences *Eunice Kennedy Shriver* National Institutes of Child Health and Human Development, National Institutes of Health, Bethesda, MD, USA
[3]The Signal Processing and Instrumentation Section, Center for Information Technology, National Institutes of Health, Bethesda, MD, USA
[4]Neuro-Oncology Branch, Center for Cancer Research, National Cancer Institute, National Institutes of Health, Bethesda, MD, USA
[5]National Institute of General Medical Sciences, National Institutes of Health, Bethesda, MD, USA

[*]peter.basser@nih.gov

# Contents


**1 Estimated media loss calculations** **3**
1.1 Mass transfer correlations and equations . . . 3
1.2 Inovitro™ device . . . 4
1.3 The present device . . . 6

**2 Heat transfer and temperature profile calculations** **9**
2.1 Assumptions, Joule heating, and boundary conditions . . . 9
2.2 Heat transfer coefficient correlations and material parameters . . . 10
2.3 Calculating combined heat transfer coefficients . . . 13
2.4 Numerical temperature profile solutions . . . 15
2.5 Internal heat fluxes and Rayleigh–Bénard convection . . . 19

**3 Image processing and threshold selection** **21**
3.1 Contrast enhancement . . . 21
3.2 Threshold selection . . . 21
3.3 Classification error correction . . . 23

# 1 Estimated media loss calculations

In this supplementary section, we explore the evaporation of cell media during EF application using empirical mass transfer correlations. The calculations are in acceptable agreement with experimental osmolarity measurements (see Table S1, Fig. 5). The calculations help to develop an intuitive understanding of what drives media loss. For example, the gas flow rate of the incubator and the exposed area of the cell media are shown to be paramount. We also estimate the media loss for the Inovitro™ device to assess the probable osmoregulation capabilities of the Inovitro™ device, and whether the present device and experimental setup offers substantially improved osmoregulation. Calculations support the conclusion that our device does, indeed, provide improved osmoregulation by over 60%.

## 1.1 Mass transfer correlations and equations

The expected media loss in from a cell culture dish can be estimated as a laminar flow convective mass transfer process. This type of problem is tackled in any transport phenomena text. For one such reference, see Ch. 28 in Ref. [1]. According to the boundary layer theory of mass transport, the molar mass transfer rate (per unit area) between the air/water vapor above the media (surface, $s$) and the surrounding fluid ($\infty$) can be expressed as

$$N_A = k_c(c_{A,s} - c_{A,\infty}), \tag{1}$$

where

$$k_c = \frac{\mathrm{Sh} D_{\mathrm{AB}}}{L}, \tag{2}$$

$\mathrm{Sh}$ is the Sherwood number, $D_{\mathrm{AB}}$ is the mass diffusivity of water vapor in 95% air, 5% $CO_2$, and $L$ is a characteristic length scale. The water vapor concentrations can be expressed in terms of the saturation pressure and the relative humidity, RH,

$$c_A = \frac{P(T)}{RT}; \quad P(T) = \mathrm{RH} \times P_{\mathrm{sat}}(T), \tag{3}$$

where $R$ is the ideal gas constant and $T$ is the temperature in Kelvin. Using the well-known correlation for the average Sherwood number over a flat dish in the case of forced convection, we have

$$\overline{\mathrm{Sh}} = 0.664\,\mathrm{Re}^{1/2}\,\mathrm{Sc}^{1/3}, \tag{4}$$

where $\mathrm{Re}$ is Reynold's number and $\mathrm{Sc}$ is Schmidt's number, defined as

$$\mathrm{Re} = \frac{U_\infty L}{\nu}; \quad \mathrm{Sc} = \frac{\nu}{D_{AB}}, \tag{5}$$

where $U_\infty$ is the velocity of the fluid far away from the dish and $\nu$ is the kinematic viscosity. The velocity can be expressed as

$$U_\infty = Q/A \tag{6}$$

where $Q$ is the volumetric flow rate and $A$ is the cross sectional area of flow. If we can determine or define all values in this set of equations, we can estimate media loss. We do so here for both the Inovitro™ device and our device. For our device, we further compare unshaped lid and shaped lid conditions as described in the main text.

## 1.2 Inovitro™ device

Let us first consider the experimental setup described for the Inovitro™ device. The concentrations can be estimated by assuming the incubator is operating at 95% RH based on practically achievable humidity levels. At the two temperatures mentioned in the Inovitro™ experiments: 37°C above the dish, and 18°C in the incubator,

$$c_{A,s}(37^\circ\mathrm{C}) = \frac{0.95P_{\mathrm{sat}}(37^\circ\mathrm{C})}{RT} = \frac{(0.95)(0.062\ \mathrm{atm})}{(0.08206\ \mathrm{L}\cdot\mathrm{atm}\cdot\mathrm{K}^{-1}\cdot\mathrm{mol}^{-1})(310.15\ \mathrm{K})} = 2.153\ \mathrm{mM}$$
$$c_{A,\infty}(18^\circ\mathrm{C}) = \frac{0.95P_{\mathrm{sat}}(18^\circ\mathrm{C})}{RT} = \frac{(0.95)(0.0204\ \mathrm{atm})}{(0.08206\ \mathrm{L}\cdot\mathrm{atm}\cdot\mathrm{K}^{-1}\cdot\mathrm{mol}^{-1})(291.15\ \mathrm{K})} = 0.811\ \mathrm{mM}$$

Using an ideal gas adjustment for STP molar volume,

$$y_{A,s} = c_{A,s}(22.4\ \mathrm{mol}\cdot\mathrm{L}^{-1})\left(\frac{310.15}{273.15}\right) = 0.0548\ \frac{\mathrm{mol\,H_2O}}{\mathrm{mol\,vap}}$$
$$y_{A,\infty} = c_{A,\infty}(22.4\ \mathrm{mol}\cdot\mathrm{L}^{-1})\left(\frac{300.65}{273.15}\right) = 0.0200\ \frac{\mathrm{mol\,H_2O}}{\mathrm{mol\,vap}}.$$

Using the diffusivity of water vapor in gasses presented in Ref. [2], the diffusivity of water vapor in the 95% air, 5 % $CO_2$ in the incubator can be estimated at the film temperature,

$$T_{\mathrm{film}} = \frac{18+37}{2} = 27.5^\circ\mathrm{C} = 300.65\,\mathrm{K},$$

as a molar average of available experimental diffusivities corrected by a $T^{3/2}$ factor (following the kinematic theory of gases),

$$\begin{aligned} D_{AB}(27.5^\circ\mathrm{C}) &\approx 0.95\left(\frac{300.65}{298.15}\right)^{\frac{3}{2}} D_{A,\mathrm{Air}}(298.15\,\mathrm{K}) + 0.05\left(\frac{300.65}{307.45}\right)^{\frac{3}{2}} D_{A,\mathrm{CO_2}}(307.45\,\mathrm{K}) \\ &= (0.95)(1.0126)(0.282\ \mathrm{cm}^2\cdot\mathrm{s}^{-1}) + (0.05)(0.9670)(0.202\ \mathrm{cm}^2\cdot\mathrm{s}^{-1}) \\ &= 0.2649\ \mathrm{cm}^2\cdot\mathrm{s}^{-1} = 2.649\times10^{-5}\ \mathrm{m}^2\cdot\mathrm{s}^{-1}. \end{aligned}$$

The kinematic viscosity of the humidified air at the film temperature can be estimated using a molar weighted average for air and $CO_2$ viscosity values. First, we determine the dynamic viscosities at the film temperature,

$$\mu_{\mathrm{CO_2}} \approx 1.516\times10^{-5};\ \ \mu_{\mathrm{Air}} \approx 1.849\times10^{-5};\ \ \mu_{\mathrm{H_2O}} \approx 9.776\times10^{-6}\ \mathrm{N}\cdot\mathrm{s}\cdot\mathrm{m}^{-2}.$$

where the value for water vapor is taken from Ref. [3] and corrected using a $T$ factor and the values for $CO_2$ and air are calculated using Sutherland's law [4]. For reference values, we use the publicly available Engineering ToolBox and Ref. [5]. Using the Herning and Zipperer [6] method for gas mixture viscosity estimates (as opposed to the more complicated Wilke method [7]; the Herning and Zipperer method should suffice for this non-polar gas mixture),

$$\begin{aligned} \mu_{\mathrm{mix}} &\approx \frac{\sum\left(\mu_i y_i\sqrt{M_i}\right)}{\sum\left(y_i\sqrt{M_i}\right)} = \frac{\mu_{\mathrm{CO_2}}y_{\mathrm{CO_2}}\sqrt{M_{\mathrm{CO_2}}} + \mu_{\mathrm{Air}}y_{\mathrm{Air}}\sqrt{M_{\mathrm{Air}}} + \mu_{\mathrm{H_2O}}y_{\mathrm{H_2O}}\sqrt{M_{\mathrm{H_2O}}}}{y_{\mathrm{CO_2}}\sqrt{M_{\mathrm{CO_2}}} + y_{\mathrm{Air}}\sqrt{M_{\mathrm{Air}}} + y_{\mathrm{H_2O}}\sqrt{M_{\mathrm{H_2O}}}} \qquad (7) \\ &= \frac{(1.516\times10^{-5})(.049)\sqrt{44} + (1.849\times10^{-5})(.931)\sqrt{29} + (9.776\times10^{-6})(.02)\sqrt{18}}{(.049)\sqrt{44} + (.931)\sqrt{29} + (.02)\sqrt{18}} \\ &= 1.815\times10^{-5}\ \mathrm{N}\cdot\mathrm{s}\cdot\mathrm{m}^{-2}. \end{aligned}$$

The mass density, assuming ideal gas behavior, is given trivially by

$$\rho \approx \frac{(.049)(44) + (.931)(29) + (.02)(18) \text{ g} \cdot \text{mol}^{-1}}{(0.0224 \text{ m}^3 \cdot \text{mol}) \left(\dfrac{300.65}{273.15}\right)} = 1.197 \text{ kg} \cdot \text{m}^{-3},$$

so that

$$\nu \approx \frac{\mu_{\text{mix}}}{\rho} = \frac{2.016 \times 10^{-5} \text{ N} \cdot \text{s} \cdot \text{m}^{-2}}{1.27 \text{ kg} \cdot \text{m}^{-3}} = 1.516 \times 10^{-5} \text{ m}^2 \cdot \text{s}^{-1}.$$

The characteristic length scale can be estimated by correcting for the circular geometry of the 35 mm culture dish, i.e., $L^2 = \pi d^2/4$, such that

$$L = L_{\text{eff}} = \frac{1}{2}\sqrt{\pi} d = \frac{1}{2}\sqrt{\pi}(0.035\,\text{m}) = 0.031\,\text{m}. \tag{8}$$

The volumetric flow rate of gas in an incubator is between 0.2 liters per minute (LPM) and 0.3 LPM, depending on the size of the incubator. Using specifications for the Thermo Scientific Heracell 150i as a representative example, the internal cross sectional area is 42.3 $\times$ 44.5 cm $= 0.188\,\text{m}^2$ and the flow rate is 0.25 LPM. A reasonable estimate for $U_\infty$ is thus

$$U_\infty = \frac{Q}{A} \approx \frac{(1/60)\ 0.2 \times 10^{-3}\,\text{m}^3 \cdot \text{s}^{-1}}{0.188\,\text{m}^2} = 2.216 \times 10^{-5}\,\text{m} \cdot \text{s}^{-1}.$$

Note, the mole fraction of water vapor is small, so $k_c$ should be corrected by a log mean concentration factor,

$$k_c \to \frac{k_c}{(1 - y_A)_{\text{lm}}} = k_c \left[ \frac{(1 - y_{A,s}) - (1 - y_{A,\infty})}{\ln\left(\dfrac{1 - y_{A,s}}{1 - y_{A,\infty}}\right)} \right]^{-1}, \tag{9}$$

and

$$(1 - y_A)_{\text{lm}} = 0.9625.$$

Now with all values in hand, the dimensionless parameters are calculated as

$$\begin{aligned}
\text{Re} &= \frac{U_\infty L}{\nu} = \frac{(2.216 \times 10^{-5}\,\text{m} \cdot \text{s}^{-1})(0.031\,\text{m})}{1.587 \times 10^{-5}\ \text{m}^2 \cdot \text{s}^{-1}} = 0.0433, \\
\text{Sc} &= \frac{\nu}{D_{AB}} = \frac{1.516 \times 10^{-5}\ \text{m}^2 \cdot \text{s}^{-1}}{2.649 \times 10^{-5}\ \text{m}^2 \cdot \text{s}^{-1}} = 0.5723, \\
\text{Sh} &= 0.664\,\text{Re}^{1/2}\,\text{Sc}^{1/3} = 0.1147, \\
k_c &= \frac{\text{Sh} D_{\text{AB}}}{L(1 - y_A)_{\text{lm}}} = \frac{(0.1147)(2.649 \times 10^{-5}\ \text{m}^2 \cdot \text{s}^{-1})}{(0.031\,\text{m})(0.9625)} = 1.018 \times 10^{-4}\ \text{m} \cdot \text{s}^{-1}.
\end{aligned}$$

Note that the extremely low value of the Reynold's number supports our laminar flow assumption. Note, also, that $\text{Sh} < 1$ indicates a diffusion-dominated mass transfer process. Finally,

$$\begin{aligned}
N_A &= k_c(c_{A,s} - c_{A,\infty}) = 1.018 \times 10^{-4}\ \text{m} \cdot \text{s}^{-1}\,(2.153 - 0.811)\ \text{mol}\,\text{H}_2\text{O} \cdot \text{m}^{-3} \\
&= 1.367 \times 10^{-4}\ \frac{\text{mol}\,\text{H}_2\text{O}}{\text{m}^2 \cdot \text{s}}.
\end{aligned}$$

The media volume lost over one day, assuming steady state conditions, is

$$V_{\text{evap}} = N_A L_{\text{eff}}^2 (3600 \cdot 24)(18.015 \text{ g} \cdot \text{mol}\,\text{H}_2\text{O}^{-1})(1 \text{ g} \cdot \text{mL}^{-1}) \approx \mathbf{0.204} \text{ mL} \cdot \text{day}^{-1}.$$

Since we have not been rigorous with certainties and significant figures in our parameter estimation, we state only that over half a milliliter of media loss can be expected over a 3 day period of stimulation if a 35 mm dish is cultured at the conditions described in the Inovitro™ device literature. A 0.61 mL loss amounts to a final $\approx 31\%$ of media volume lost (or **44**% increase in osmolarity) if using the typical 2 mL of media in a 35 mm dish. The osmolarity change is calculated assuming no solute loss, so that the percentage change is given by

$$\% \text{ change in osmolarity} = \left[ \frac{2 \text{ mL}}{(2 - V_{\text{evap}}) \text{ mL}} - 1 \right] \times 100. \tag{10}$$

The fact that the Inovitro™ literature calls for media replacement every day during the experiment is reasonable to avoid hyperosmolar bath conditions. However, rapid vacillations in osmolarity conditions can cause adverse effects on cells, as mentioned in the Introduction.

## 1.3 The present device

We now repeat the calculations for our system for the various experimental setups described in the text. The media surface condition should be the same as the previous calculations, but the surrounding air conditions are different. The temperature of the air around the coil is approximately 22°C at the middle of the 72 h experiment, giving a new film temperature of

$$T_{\text{film}} = \frac{22 + 37}{2} = 29.5^\circ\text{C} = 302.65 \text{ K}.$$

Recalculating all affected parameters,

$$c_{A,\infty}(22^\circ\text{C}) \approx \frac{(0.95)P_{\text{sat}}(29.5^\circ\text{C})}{RT} = \frac{0.95(0.0261 \text{ atm})}{(0.08206)(293.15)} = 1.024 \text{ mM},$$

$$y_{A,\infty} = c_{A,\infty}(22.4 \text{ mol} \cdot \text{L}^{-1}) \left( \frac{295.15}{273.15} \right) = 0.0248 \ \frac{\text{mol}\,\text{H}_2\text{O}}{\text{mol}\,\text{vap}},$$

$$\begin{aligned} D_{AB}(29.5^\circ\text{C}) &\approx 0.95 \left( \frac{302.65}{298.15} \right)^{\frac{3}{2}} D_{A,\text{Air}}(298.15\,\text{K}) + 0.05 \left( \frac{302.65}{307.45} \right)^{\frac{3}{2}} D_{A,\text{CO}_2}(307.45\,\text{K}) \\ &= (0.95)(1.023)(0.282 \text{ cm}^2 \cdot \text{s}^{-1}) + (0.05)(0.9757)(0.202 \text{ cm}^2 \cdot \text{s}^{-1}) \\ &= 0.2838 \text{ cm}^2 \cdot \text{s}^{-1} = 2.838 \times 10^{-5} \text{ m}^2 \cdot \text{s}^{-1}, \end{aligned}$$

$$\mu_{\text{CO}_2} \approx 1.503 \times 10^{-5}; \ \ \mu_{\text{Air}} \approx 1.858 \times 10^{-5}; \ \ \mu_{\text{H}_2\text{O}} \approx 9.849 \times 10^{-6} \text{ N} \cdot \text{s} \cdot \text{m}^{-2},$$

$$\begin{aligned} \mu &\approx \frac{(1.503 \times 10^{-5})(.0492)\sqrt{44} + (1.858 \times 10^{-5})(.926)\sqrt{29} + (9.849 \times 10^{-6})(.0248)\sqrt{18}}{(.0492)\sqrt{44} + (.926)\sqrt{29} + (.0248)\sqrt{18}} \\ &= 1.820 \times 10^{-5} \text{ N} \cdot \text{s} \cdot \text{m}^{-2}, \end{aligned}$$

$$\rho \approx \frac{(.0492)(44) + (.926)(29) + (.0248)(18) \text{ g} \cdot \text{mol}^{-1}}{(0.0224 \text{ m}^3 \cdot \text{mol}) \left( \frac{302.65}{273.15} \right)} = 1.187 \text{ kg} \cdot \text{m}^{-3},$$

$$\nu \approx \frac{1.820 \times 10^{-5}\ \mathrm{N \cdot s \cdot m^{-2}}}{1.187\ \mathrm{kg \cdot m^{-3}}} = 1.533 \times 10^{-5}\ \mathrm{m^2 \cdot s^{-1}},$$

$$(1 - y_A)_{\mathrm{lm}} = 0.9601$$

Then, for the flat lid condition (which as the same effective $L$),

$$\begin{aligned}
\mathrm{Re} &= \frac{U_\infty L}{\nu} = \frac{(2.216 \times 10^{-5}\,\mathrm{m \cdot s^{-1}})(0.031\,\mathrm{m})}{1.555 \times 10^{-5}\ \mathrm{m^2 \cdot s^{-1}}} = 0.0442,\\
\mathrm{Sc} &= \frac{\nu}{D_{AB}} = \frac{1.533 \times 10^{-5}\ \mathrm{m^2 \cdot s^{-1}}}{2.838 \times 10^{-5}\ \mathrm{m^2 \cdot s^{-1}}} = 0.5403,\\
\overline{\mathrm{Sh}} &= 0.664\,\mathrm{Re}^{1/2}\,\mathrm{Sc}^{1/3} = 0.1137,\\
k_c &= \frac{\mathrm{Sh} D_{\mathrm{AB}}}{L(1 - y_A)_{\mathrm{lm}}} = \frac{(0.1137)(2.838 \times 10^{-5}\ \mathrm{m^2 \cdot s^{-1}})}{(0.031\,\mathrm{m})(0.9601)} = 1.084 \times 10^{-4}\ \mathrm{m \cdot s^{-1}},\\
N_A &= k_c(c_{A,s} - c_{A,\infty}) = 1.084 \times 10^{-4}\ \mathrm{m \cdot s^{-1}}\,(2.153 - 1.024)\ \mathrm{mol\,H_2O \cdot m^{-3}}\\
&= 1.224 \times 10^{-4}\ \frac{\mathrm{mol\,H_2O}}{\mathrm{m^2 \cdot s}},
\end{aligned}$$

and finally,

$$V_{\mathrm{evap}} = N_A L_{\mathrm{eff}}^2 (3600 \cdot 24)(18.015\ \mathrm{g \cdot mol\,H_2O^{-1}})(1\ \mathrm{g \cdot mL^{-1}}) = \mathbf{0.183}\ \mathrm{mL \cdot day^{-1}},$$

resulting in approximately 0.55 mL media loss over the course of a 3 day experiment. This amounts to a 27% loss of media and a **38%** increase in osmolarity. These values are in relatively close agreement with our measured osmolarity changes in Fig. 5. Using a vapor osmometer, we had measured an $\approx 39 \pm 8\%$ (1 SD from 3 measurements) increase in osmolarity for this condition. In 3 mL, 0.55 mL loss would result in 22% increase in osmolarity, which is less similar to our experimentally measured increase of $33 \pm 6\%$.

While these estimates are in reasonable agreement with measurements, some discrepancies between model and measurements may arise from: (1) unaccounted for re-condensation of media on the interior of the dish, (2) the fact that the local coil air temperature differs from the surrounding incubator air temperature (introducing a second, further boundary condition and mass transfer process), or (3) failure of certain model assumptions. Notably, the Schmidt number of 0.54 is less than the heuristic 0.6 lower limit for the correlations used. The incubator is also an imperfectly closed system as evidenced by media loss even in the control condition; the RH at the edge of the incubator might drop precipitously. We have also ignored any temperature gradients within the dish which, naturally, lead to vapor pressure gradients.

Nonetheless, our measurements and our calculations demonstrate that without any mitigation measures, our device has similarly poor osmoregulation compared to the Inovitro™ device due to the cool, 22°C surrounding air temperature. Mitigation techniques are necessary. Recall, the mitigation techniques involved lid shaping and using a larger volume of media. Only the former, lid shaping, changes any parameters: $L_{\mathrm{eff}}$ is reduced. This reduction in area is illustrated in Fig. S1 below.

The outer diameter is still 35 mm; the effective inner diameter becomes $\approx 21.9$ mm. Using the remaining area to calculate a new effective length scale,

$$L_{\mathrm{eff}} = \sqrt{\frac{\pi(0.035\ \mathrm{m})^2}{4} - \frac{\pi(0.0219\ \mathrm{m})^2}{4}} = 0.0242\ \mathrm{m}$$

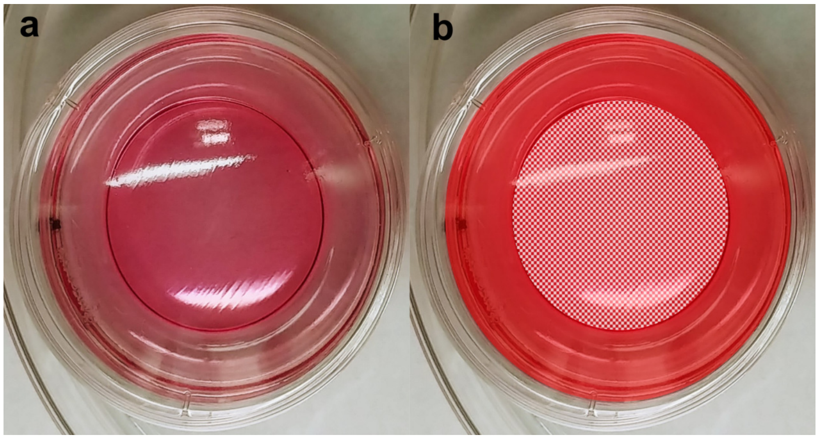


**Figure S1:** Schematic of area reduction from lid modification. Photo of shaped lid (**a**) with shaded areas (**b**). Area exposed to air shown in red.

**Table S1.** Estimated and measured percentage changes in osmolarity after 3 days stimulation.

| Condition | Estimated Osmol. $\Delta(\%)$ | Measured Osmol. $\Delta(\%)$ |
|---|---|---|
| Inovitro ™ device | 44 | - |
| Treated, Flat Lid, 2 mL | 38 | $39 \pm 8$ |
| Treated, Flat Lid, 3 mL | 22 | $33 \pm 6$ |
| Treated, Curved Lid, 2 mL | 23 | - |
| Treated, Curved Lid, 3 mL | 14 | $17 \pm 4$ |

Now recalculating all values affected by this parameter change,

$$\begin{aligned}
\mathrm{Re} &= \frac{U_\infty L}{\nu} = \frac{(2.216\times10^{-5}\,\mathrm{m\cdot s^{-1}})(0.0242\,\mathrm{m})}{1.558\times10^{-5}\ \mathrm{m^2\cdot s^{-1}}} = 0.03442,\\
\overline{\mathrm{Sh}} &= 0.664\,\mathrm{Re}^{1/2}\,\mathrm{Sc}^{1/3} = 0.1003,\\
k_c &= \frac{\mathrm{Sh}D_{\mathrm{AB}}}{L(1-y_A)_{\mathrm{lm}}} = \frac{(0.1003)(2.838\times10^{-5}\ \mathrm{m^2\cdot s^{-1}})}{(0.0242\,\mathrm{m})(0.9601)} = 1.226\times10^{-4}\ \mathrm{m\cdot s^{-1}},\\
N_A &= k_c(c_{A,s}-c_{A,\infty}) = 1.226\times10^{-4}\ \mathrm{m\cdot s^{-1}}\ (2.153-1.024)\ \mathrm{mol\,H_2O\cdot m^{-3}}\\
&= 1.384\times10^{-4}\ \frac{\mathrm{mol\,H_2O}}{\mathrm{m^2\cdot s}},
\end{aligned}$$

and,

$$V_{\mathrm{evap}} = N_A L_{\mathrm{eff}}^2(3600\cdot24)(18.015\ \mathrm{g\cdot mol\,H_2O^{-1}})(1\ \mathrm{g\cdot mL^{-1}}) = \mathbf{0.126}\ \mathrm{mL\cdot day^{-1}},$$

which is a 31% reduction in media loss from the unshaped lid condition. Over 3 days, about 0.38 mL media loss is expected. In 2 mL, this amounts to a **23**% increase in final osmolarity. In 3 mL, a **14**% increase in final osmolarity is expected. This prediction is in good agreement with our experimental measurements of $17 \pm 4\%$ osmolarity increase after 3 days of stimulation for the curved, 3 mL condition.

A summary of osmolarity increase estimations and measurements is shown in Table S1. Overall, estimations are in acceptable agreement with measurements, except, notably, the flat 3 mL condition. Observed agreement supports the validity of the simplified mass transfer models used here. Therefore, our estimation of media loss in the Inovitro™ device should be reasonable. Our estimates indicate that media loss and the resulting osmolarity increase is a major challenge for any cell culture device operating in a refrigerated environment with an appreciable gas flow rate. This is more of a challenge for the Inovitro ™ device than our device due to the lower surrounding operating temperatures (18 vs. 22°C) and the lack of mitigation strategies.

# 2 Heat transfer and temperature profile calculations

A deeper understanding of the heat transfer mechanisms alluded to in Fig. 4 is developed here. We perform theoretical calculations for the approximate steady state temperature profiles that should develop for our experimental conditions. We develop reasonable assumptions and solve the resulting heat equation numerically. For an introduction to the convective heat transfer principles employed here, see Ch. 17, 19 – 20 in [1] or Ch. 14 in Ref. [8].

## 2.1 Assumptions, Joule heating, and boundary conditions

We *ignore heat transfer between adjacent dishes and then out to the environment*, reasoning that the compound thermal resistance through two different sets of dish materials is extremely large compared to the thermal resistances within and adjacent to a single dish, especially given the small temperature gradients between dishes. This is the only major simplifying assumption. All other sources of heat transfer are considered.

One source of heat transfer is radiation to the surroundings,

$$\dot{q}_{\mathrm{rad}} = \epsilon\sigma(T^4 - T^4_{\mathrm{ambient}})A,$$

where $\epsilon$ is the emissivity coefficient of the media, $\sigma$ here is the Stefan-Boltzmann constant, and $A$ is total the media surface area. Here, the sleeve will absorb most of the radiation such that the ambient temperature is the temperature of the sleeve. The sleeve, in turn, is assumed to be in equilibrium with the cooler air around the coil so $T_{\mathrm{ambient}} = T_{\mathrm{coil}} = T_\infty$. The other sources of heat transfer and generation are captured in the heat partial differential equation (PDE) without radiation,

$$\rho c_p \frac{\partial T(x,y,z,t)}{\partial t} = k\nabla^2 \cdot T(x,y,z,t) + \underline{\dot{q}}, \tag{11}$$

where $c_p$ is the isobaric heat capacity, $\rho$ is the mass density, $T$ is temperature, $k$ is the thermal conductivity, and $\underline{\dot{q}}$ is the rate of heat generation per volume and can be a function of space and time. The internal heat generation can be expressed as volumetric power generation due to Joule heating for our system. As discussed in the main text, Joule heating is a function of radius by

$$\begin{gathered}\underline{\dot{q}}(r) = \frac{P_{\mathrm{total}}(r)}{V(r)} = \frac{\pi\sigma L_z m^2 r^4}{16} \times \frac{1}{\pi r^2 L_z} = \frac{\sigma m^2 r^2}{16} \\ m := \frac{\mu_0}{2}\left(\frac{N}{L}\right)\left|\frac{dI}{dt}\right|_{\mathrm{pk-pk}}.\end{gathered} \tag{12}$$

The heat equation can be reduced to two dimensions by symmetry. Assuming no $\theta$ dependency,

$$\rho c_p \frac{\partial T(r,\theta,t)}{\partial t} = k\left[\frac{1}{r}\frac{\partial}{\partial r}\left(r\frac{\partial T}{\partial r}\right) + \frac{\partial^2 T}{\partial z^2}\right] + \frac{\sigma m^2 r^2}{16} \tag{13}$$

We next define boundary conditions to solve the problem. The boundary conditions are convective. The cell media is in contact with the dish and the dish is in contact with the cold air surrounding the coil. We can treat this as a composite wall and compute effective heat transfer coefficients,

$$-k\frac{dT(R,t)}{dr} = U[T(R,t) - T_\infty] \tag{14}$$

where $R$ is the dish radius, $k$ is the thermal conductivity of the media, $U$ is the effective heat transfer coefficient through the cell media-dish-air-sleeve composite wall(s), and $T_\infty$ is the ambient (coil) temperature. The cell media can be considered as a cylinder, with each of its faces experiencing a different convective heat transfer boundary condition.

## 2.2 Heat transfer coefficient correlations and material parameters

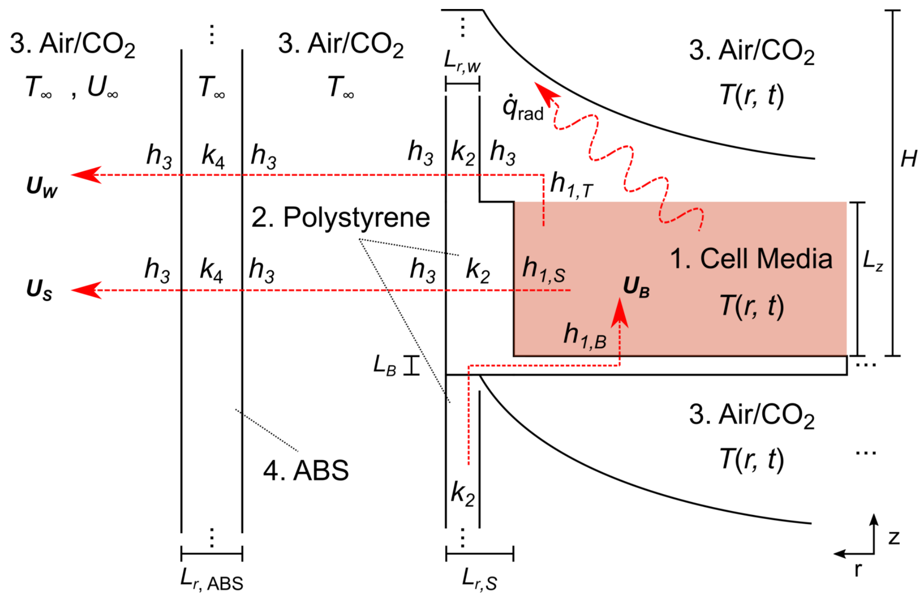


**Figure S2:** Schematic diagram of the single dish heat transfer problem. Cell media (1) in contact with a polystyrene dish wall (2) at $r = R$. The wall is in contact with cool air (3) that is then in contact, for some part of the stack, with (4) ABS plastic. Air beyond the wall has a flow rate and temperature of $U_\infty$ and $T_\infty$, respectively. Warm air rests above the media inside the dish. Two parallel heat transfer pathways from the side, $S$, and top, $T$, of the media are shown with labelled substituent heat transfer coefficients. The pathway through the top, or surface, leaves through the wall, $W$. An additional heat transfer pathway comes through the dish bottom, $B$. Directly above and below the dish is air trapped in the domed lid area(s), measured to be at the same temperature as the media and thus not contributing any significant heat transfer. Radiation heat transfer is also illustrated. Relevant lengths are labelled.

At the dish boundary, we have an interface with 3 materials: (1) cell medium, (2) polystyrene dish wall, and (3) humidified air. Farther, we have the plastic sleeve (4). These numeric designations will be used to subscript all coefficients. For clarification of dimensions and components, a schematic diagram is shown below in Fig. S2.

$U_S$, the effective heat transfer coefficient from the side ($S$) of the media, is given by a summation of two series of heat transfer coefficients: one that incorporates the acrylonitrile butadiene styrene (ABS) dish stack holder and

one that does not, reflecting the gaps in the stack holder (see Figs. 1a and b). According to measurements, 28.8% of the circumference of the dish stack holder is open such that

$$U_S = 0.288\left(\frac{L_{r,S}}{k_2} + \frac{1}{h_{1,S}} + \frac{1}{h_3}\right)^{-1} + 0.712\left(\frac{L_{r,S}}{k_2} + \frac{1}{h_{1,S}} + \frac{L_{r,\mathrm{ABS}}}{k_4} + \frac{3}{h_3}\right)^{-1} \ \mathrm{W}\cdot\mathrm{m}^{-2}\cdot\mathrm{K}^{-1}, \tag{15}$$

Above the media, heat transfer between the warm air along the dish wall (*W*) and the cold air occurs. Again, we account for the pathway through ABS and the pathway direct to air. Further complicating this term, area correction needs to be applied,

$$U_W = \frac{0.288}{A_S}\left(\frac{1}{A_S h_{1,T}} + \frac{L_{r,T}}{A_W k_2} + \frac{2}{A_W h_3}\right)^{-1} + \frac{0.712}{A_S}\left(\frac{1}{A_S h_{1,T}} + \frac{L_{r,T}}{A_W k_2} + \frac{L_{r,\mathrm{ABS}}}{A_W k_4} + \frac{4}{A_W h_3}\right)^{-1} \ \mathrm{W}\cdot\mathrm{m}^{-2}\cdot\mathrm{K}^{-1}, \tag{16}$$

where $A_W$ is the area of the dish wall above the media and $A_S$ is the media surface area. At the bottom (*B*) of the dish, we have a domed lid that reduces the conducting surface between the bottom of the dish and the lid of the dish below. The area reduction can be estimated using the wall thickness, $L_{r,S}$ and a contact rim of 0.5 mm, $\dfrac{\Delta A}{A} = 1 - \dfrac{R_o^2 - R_i^2}{R_o^2} \approx 94.4\%$ so that an appropriate corrective factor can be applied. We assume that the dish walls are in contact down to the Plexiglas shelf, such that the ambient temperature for the bottom surface is the incubator temperature, rather than the coil temperature

$$U_B = \left(17.8\frac{L_B}{k_2} + \frac{1}{h_{1,B}}\right)^{-1} \ \mathrm{W}\cdot\mathrm{m}^{-2}\cdot\mathrm{K}^{-1}. \tag{17}$$

We now assess material parameters at the film temperature, which is again

$$T_{\mathrm{film}} = \frac{22+37}{2} = 29.5^\circ\mathrm{C} = 302.65\ \mathrm{K},$$

Obviously,

$$\Delta T = T - T_\infty \approx 37 - 22 = 15\ \mathrm{K}.$$

The parameters for the polystyrene dish are as follows: measured thickness of 1.7 mm near the base and along the bottom, and 1 mm further from the base,

$$L_{r,S} = L_B = 1.7\ \mathrm{mm};\ \ L_{r,W} = 1\ \mathrm{mm},$$
$$k_2 \approx 0.22\ \mathrm{W}\cdot\mathrm{m}^{-1}\cdot\mathrm{K}^{-1}\ @\,23^\circ\mathrm{C},$$

where the thermal conductivity is the value for high impact polystyrene thermal characteristics from Ref. [9]. For ABS, we have

$$L_{r,\mathrm{ABS}} = 3.5\ \mathrm{mm};\ k_4 \approx 0.175\ \mathrm{W}\cdot\mathrm{m}^{-1}\cdot\mathrm{K}^{-1}\ @\,23^\circ\mathrm{C}.$$

With expressions and plastic parameters now defined, we turn towards describing the relevant correlations and fluid parameters.

Following Ch. 20 in Ref. [1], the correlations for the heat transfer coefficient for cylinders horizontal to external flow are given by Churchill and Chu [10] as

$$h = \frac{k}{D}\left(0.6 + \frac{0.387\mathrm{Ra}_D^{1/6}}{\left[1+(0.559\mathrm{Pr})^{9/16}\right]^{8/27}}\right)^2 \quad \text{for } 10^{-5} < \mathrm{Ra}_D < 10^{12}, \tag{18}$$

where $D$ is the cylinder diameter, $\mathrm{Ra}_D$ is the diameter-wise Rayleigh number, Pr is the Prandtl number, and $k$ is the thermal conductivity of the fluid. The Prandtl number is

$$\mathrm{Pr} = \frac{c_p\mu}{k}, \tag{19}$$

where $\mu$ is the dynamic viscosity, and the Rayleigh number is,

$$\mathrm{Ra}_D = \mathrm{Pr}\mathrm{Gr}_D, \tag{20}$$

$\mathrm{Gr}_D$ is the Grashof number,

$$\mathrm{Gr}_D = \frac{g(T_s - T_\infty)\beta D^3}{\nu^2}, \tag{21}$$

$\nu$ is the dynamic viscosity, $\beta$ is the coefficient of linear thermal expansion ($\approx 1/T$ for ideal gases), $g$ is gravitational acceleration ($= 9.81\ \mathrm{m}\cdot\mathrm{s}^{-2}$), and all Prandtl and Grashof number parameters are for the fluid. This correlation is used to find $h_{1,S}$, and $h_3$. For $h_{1,T}$, the relevant geometry is not a horizontal cylinder, but a horizontal plane. The appropriate correlation for a flat hot surface facing up, according to McAdams [11], is,

$$h = \frac{0.54k\mathrm{Ra}_L^{1/4}}{L},\ L = \frac{\text{surface area}}{\text{perimeter}} = \frac{R}{2} \quad \text{for} \quad 10^5 < \mathrm{Ra}_L < 2\times10^7 \tag{22}$$

For the cell media, we consider its thermal properties to be very close to those of water at the film temperature, so according to readily available properties of water, linearly interpolated where necessary,

$$\begin{aligned}
&\text{water @ } 302.65\,\mathrm{K}:\\
k &= 0.614\ \mathrm{W}\cdot\mathrm{m}^{-1}\cdot\mathrm{K}^{-1}\\
c_p &= 4.18\ \mathrm{kJ}\cdot\mathrm{kg}^{-1}\cdot\mathrm{K}^{-1}\\
\mu &= 8.055\times10^{-4}\ \mathrm{N}\cdot\mathrm{s}\cdot\mathrm{m}^{-2}\\
\rho &= 995.82\ \mathrm{kg}\cdot\mathrm{m}^{-3}\\
\beta &= 2.984\times10^{-4}\ \mathrm{K}^{-1}.
\end{aligned}$$

For the air/$CO_2$ mixture we previously obtained viscosity and density estimates at this film temperature. Other parameters can be estimated from mass-weighted averages (recall, $y_{\mathrm{H_2O}} = 0.0248$) of available reference values [5], linearly interpolated where necessary,

$$\begin{aligned}
&\text{Humidified Air/CO}_2 \text{ @ } 302.65\,\mathrm{K}:\\
k &\approx \frac{y_{\mathrm{CO_2}}M_{\mathrm{CO_2}}k_{\mathrm{CO_2}} + y_{\mathrm{Air}}M_{\mathrm{Air}}k_{\mathrm{Air}} + y_{\mathrm{H_2O}}M_{\mathrm{H_2O}}k_{\mathrm{H_2O}}}{y_{\mathrm{CO_2}}M_{\mathrm{CO_2}} + y_{\mathrm{Air}}M_{\mathrm{Air}} + y_{\mathrm{H_2O}}M_{\mathrm{H_2O}}}\ \mathrm{W}\cdot\mathrm{m}^{-1}\cdot\mathrm{K}^{-1}\\
&= \frac{(0.0492)(44)(0.0170) + (0.926)(29)(0.0264) + (0.0248)(18)(0.0189)}{(0.0492)(44) + (0.926)(29) + (0.0248)(18)}\\
&= 0.0256\ \mathrm{W}\cdot\mathrm{m}^{-1}\cdot\mathrm{K}^{-1}\\
c_p &\approx \frac{(0.0492)(44)(0.844) + (0.926)(29)(1.005) + (0.0248)(18)(1.864)}{(0.0492)(44) + (0.926)(29) + (0.0248)(18)}\\
&= 1.006\ \mathrm{kJ}\cdot\mathrm{kg}^{-1}\cdot\mathrm{K}^{-1}
\end{aligned}$$

Lastly, $L_z$ can be estimated from the height of 3 mL media in a dish of 35 mm. Note that our film temperature is picked from roughly the middle of experiments (see Fig. 2), after some media has already evaporated. From the previous section, we can estimate that by the time the present film temperature is achieved, the media has decreased by 0.147 mL/day × 1.5 days = 0.2205 mL to 2.7795 mL, so

$$L_z \approx (2779.5 \text{ mm}^3)/(35 \times 35 \text{ mm}^2) = 2.269 \text{ mm} = 2.269 \times 10^{-3} \text{ m},$$

From a 10 mm total dish height, we have that

$$H - L_z = 7.31 \times 10^{-3} \text{ m}.$$

## 2.3 Calculating combined heat transfer coefficients

Let us first calculate the constituent coefficients for the cell media. Calculating the free convection coefficient to the wall for the cell media, $h_{1,S}$,

$$\begin{aligned}
\text{Pr} &= \frac{c_p \mu}{k} = \frac{(4.18 \times 10^3 \text{ J} \cdot \text{kg}^{-1} \cdot \text{K}^{-1})(8.055 \times 10^{-4} \text{ N} \cdot \text{s} \cdot \text{m}^{-2})}{0.614 \text{ W} \cdot \text{m}^{-1} \cdot \text{K}^{-1}} \\
&= 5.484 \\
\text{Gr}_D &= \frac{g(T_s - T_\infty)\beta D^3}{(\mu/\rho)^2} = \frac{(9.81 \text{ m} \cdot \text{s}^{-2})(15 \text{ K})(2.984 \times 10^{-4} \text{ K}^{-1})(3.5 \times 10^{-2} \text{ m})^3}{(8.055 \times 10^{-4} \text{ N} \cdot \text{s} \cdot \text{m}^{-2}/995.82 \text{ kg} \cdot \text{m}^{-3})^2} \\
&= 2.877 \times 10^6 \\
\text{Ra}_D &= \text{Pr}\text{Gr}_D = (5.484)(2.877 \times 10^6) = 1.578 \times 10^7 \\
h_{1,S} &= \frac{k}{D}\left(0.6 + \frac{0.387\text{Ra}_D^{1/6}}{\left[1 + (0.559\text{Pr})^{9/16}\right]^{8/27}}\right)^2 \\
&= \frac{(0.614 \text{ W} \cdot \text{m}^{-1} \cdot \text{K}^{-1})}{(3.5 \times 10^{-2} \text{ m})}\left(0.68 + \frac{\left[(0.387)(1.578 \times 10^7)\right]^{1/6}}{\{1 + [(0.559)(5.484)]^{9/16}\}^{8/27}}\right)^2 \\
&= 1958 \text{ W} \cdot \text{m}^{-2} \cdot \text{K}^{-1}.
\end{aligned}$$

For the bottom of the dish and assuming a 1 degree difference, $h_{1,B}$ is calculated as

$$\begin{aligned}
\text{Pr} &= \frac{(4.18 \times 10^3 \text{ J} \cdot \text{kg}^{-1} \cdot \text{K}^{-1})(6.965 \times 10^{-4} \text{ N} \cdot \text{s} \cdot \text{m}^{-2})}{0.624 \text{ W} \cdot \text{m}^{-1} \cdot \text{K}^{-1}} = 4.666, \\
\text{Gr}_L &= \frac{(9.81 \text{ m} \cdot \text{s}^{-2})(1 \text{ K})(3.606 \times 10^{-4} \text{ K}^{-1})(0.0175/2 \text{ m})^3}{(6.965 \times 10^{-4} \text{ N} \cdot \text{s} \cdot \text{m}^{-2}/993.2 \text{ kg} \cdot \text{m}^{-3})^2} \\
&= 4819, \\
\text{Ra}_L &= \text{Pr}\text{Gr}_L = (4.666)(4819) = 2.249 \times 10^4 \\
h_{1,B} &= \frac{0.54(0.624 \text{ W} \cdot \text{m}^{-1} \cdot \text{K}^{-1})(2.249 \times 10^4)^{1/4}}{(0.0175/2) \text{ m}} \\
&= 471.6 \text{ W} \cdot \text{m}^{-2} \cdot \text{K}^{-1}.
\end{aligned}$$

Now on to the calculations for the air mixture heat transfer coefficients. For $h_{1,T}$, consider that the doming of the lid reduces the effective length scale. The surface area to perimeter ratio of the area described in Fig. S1 is

$L_{\mathrm{eff}} = 3.275 \times 10^{-3}$ m so that

$$\begin{aligned}
\mathrm{Pr} &= \frac{(1006\ \mathrm{J \cdot kg^{-1} \cdot K^{-1}})(1.820 \times 10^{-5}\ \mathrm{N \cdot s \cdot m^{-2}})}{0.0256\ \mathrm{W \cdot m^{-1} \cdot K^{-1}}} = 0.7152, \\
\mathrm{Gr}_L &= \frac{g(T_s - T_\infty)\beta L_{\mathrm{eff}}^3}{(\mu/\rho)^2} = \frac{(9.81\ \mathrm{m \cdot s^{-2}})(15\ \mathrm{K})(3.304 \times 10^{-3}\ \mathrm{K^{-1}})(3.275 \times 10^{-3}\ \mathrm{m})^3}{(1.533 \times 10^{-5}\ \mathrm{m^2 \cdot s^{-1}})^2} \\
&= 72.67, \\
\mathrm{Ra}_L &= \mathrm{Pr}\mathrm{Gr}_L = (0.7152)(72.67) = 51.97, \\
h_{1,T} &= \frac{0.54 k \mathrm{Ra}_L^{1/4}}{L_{\mathrm{eff}}} = \frac{(0.54)(0.0256\ \mathrm{W \cdot m^{-1} \cdot K^{-1}})(51.97)^{1/4}}{(3.275 \times 10^{-3}\ \mathrm{m})} \\
&= 11.33\ \mathrm{W \cdot m^{-2} \cdot K^{-1}}.
\end{aligned}$$

For $h_3$, the Prandtl number is identical. For the characteristic length, we use an intermediate diameter between the various surfaces for which we apply the same approximate $h_3$ (see Fig. S2), assuming $D \approx 3.7$ cm,

$$\begin{aligned}
\mathrm{Gr}_D &= \frac{(9.81\ \mathrm{m \cdot s^{-2}})(15\ \mathrm{K})(3.304 \times 10^{-3}\ \mathrm{K^{-1}})(3.7 \times 10^{-2}\ \mathrm{m})^3}{(1.533 \times 10^{-5}\ \mathrm{m^2 \cdot s^{-1}})^2} = 1.048 \times 10^5, \\
\mathrm{Ra}_D &= (1.048 \times 10^5)(0.7152) = 7.495 \times 10^4 \\
h_3 &= \frac{(0.0256\ \mathrm{W \cdot m^{-1} \cdot K^{-1}})}{(3.7 \times 10^{-2}\ \mathrm{m})} \left(0.6 + \frac{\left[(0.387)(7.495 \times 10^4)\right]^{1/6}}{\{1 + [(0.559)(0.7152)]^{9/16}\}^{8/27}}\right)^2 \\
&= 20.36\ \mathrm{W \cdot m^{-2} \cdot K^{-1}}.
\end{aligned}$$

There is also forced convection within the incubator, as discussed in the previous section. However, considering the Richardson number, $\mathrm{Ri} = \mathrm{Gr}_D/\mathrm{Re}^2 \gg 10$, the forced component is negligible compared to the natural convection component calculated above and can be ignored.

The overall heat transfer coefficient through the composite material layer adjacent to the media is thus

$$\begin{aligned}
U_S = 0.288 &\left(\frac{L_{r,S}}{k_2} + \frac{1}{h_{1,S}} + \frac{1}{h_3}\right)^{-1} + \\
0.712 &\left(\frac{L_{r,S}}{k_2} + \frac{1}{h_{1,S}} + \frac{L_{r,\mathrm{ABS}}}{k_4} + \frac{3}{h_3}\right)^{-1}\ \mathrm{W \cdot m^{-2} \cdot K^{-1}} \\
= 0.288 &\left(\frac{0.0017}{0.22} + \frac{1}{1958} + \frac{1}{20.36}\right)^{-1} + \\
0.712 &\left(\frac{0.0017}{0.22} + \frac{1}{1958} + \frac{0.0035}{0.175} + \frac{3}{20.36}\right)^{-1} \\
= \mathbf{9.08}&\ \mathrm{W \cdot m^{-2} \cdot K^{-1}}.
\end{aligned}$$

Expectedly, the boundary heat transfer is limited principally by the slow convection between the wall and the air.

**Table S2.** Estimated heat transfer coefficients.

| Surface, coefficient | Value ($\mathrm{W \cdot m^{-2} \cdot K^{-1}}$) | Ambient temperature (°C) |
|---|---|---|
| Bottom of dish, $U_B$ | 12.04 | 37 |
| Side of dish, $U_S$ | 9.08 | 22 |
| Top of media, $U_W$ | 3.52 | 22 |

For $U_W$ (note, $A_S = 9.621 \times 10^{-4}\ \mathrm{m}^2$, and $A_W = 2\pi D(H - L_z) = 8.038 \times 10^{-4}\ \mathrm{m}^2$),

$$\begin{aligned}
U_W &= \frac{0.288}{A_S}\left(\frac{1}{A_S h_{1,T}} + \frac{L_{r,W}}{A_W k_2} + \frac{2}{A_W h_3}\right)^{-1} + \\
&\quad \frac{0.712}{A_S}\left(\frac{1}{A_S h_{1,T}} + \frac{L_{r,W}}{A_W k_2} + \frac{L_{r,\mathrm{ABS}}}{A_W k_4} + \frac{4}{A_W h_3}\right)^{-1} \\
&= \frac{0.288}{A_S}\left(\frac{1}{A_S(11.33)} + \frac{0.001}{A_W(0.22)} + \frac{2}{A_W(20.36)}\right)^{-1} + \\
&\quad \frac{0.712}{A_S}\left(\frac{1}{A_S(11.33)} + \frac{0.001}{A_W(0.22)} + \frac{0.0035}{A_W(0.175)} + \frac{4}{A_W(20.36)}\right)^{-1} \\
&= \mathbf{3.52}\ \mathrm{W \cdot m^{-2} \cdot K^{-1}}.
\end{aligned}$$

And lastly,

$$U_B = \left(17.8\frac{L_B}{k_2} + \frac{1}{h_{1,B}}\right)^{-1} = \left(\frac{0.0178}{0.22} + \frac{1}{471.6}\right)^{-1} = \mathbf{12.04}\ \mathrm{W \cdot m^{-2} \cdot K^{-1}}.$$

The estimated effective heat transfer coefficients are summarized in Table S2.

## 2.4 Numerical temperature profile solutions

Before solving for the temperature profile, we need a numeric expression for the radially dependent internal heat generation. The conductivity of DMEM at culturing temperatures, as reported in Refs. [12,13] is $\sigma \approx 1.4\ \mathrm{S \cdot m^{-1}}$, though $1.5\ \mathrm{S \cdot m^{-1}}$ is reported elsewhere [14]. We unfortunately do not have our own conductivity measurement. Note that the conductivity should exhibit some frequency dependence, but not very much in the $10^5$ range here [13]. We ignore any frequency dependent effects on conductivity and use an approximate value of $1.45\ \mathrm{S \cdot m^{-1}}$. From Eq. (12)

$$\underline{\dot{q}}(r) = \frac{\sigma m^2 r^2}{16} = \frac{(1.45\ \mathrm{S \cdot m^{-1}})(4.244 \times 10^4\ \mathrm{V \cdot m^{-2}})^2}{16} = (1.632 \times 10^8)\, r^2\ \mathrm{W \cdot m^{-3}} \tag{23}$$

Integrating over the radius yields total Joule heating per plate of $0.11$ W, as mentioned in the main text. Another quantity we have not yet specified is the emissivity of the media for radiation heat transfer. We assume an approximate value of $\epsilon \approx 0.96$. We assume the relevant radiation ambient temperature is the coil temperature. Further, we assume that radiation heat transfer is only significant from the side of the dish.

All values in hand, we move to finding numerical PDE solutions under the described conditions. We use the thermal model solvers in the PDE package within MATLAB 2019a and provide all code, but a similar analysis could be performed with any reasonably capable PDE solver and finite element mesh generator. Indeed, interfacing the COMSOL electroquasistatics and heat transfer modules would provide greater resolution. We first initialize the geometry and the model, shown in Fig. S3.

```
thermalmodel = createpde('thermal');

Ro = 0.0175; % Radius [=] m
Ri = 0.01095; % Occluded by lid, see Fig. S1
Lz = 2.269E-3; % Height [=] m
g = multicylinder([Ri Ro], Lz);
thermalmodel.Geometry = g;

figure
pdegplot(thermalmodel,'EdgeLabels','off','FaceLabels','on', ...
                      'FaceAlpha', 0.25)

figure
msh = generateMesh(thermalmodel, 'Hmax', 0.001); % Max 1 mm triangle height
pdemesh(msh);
```

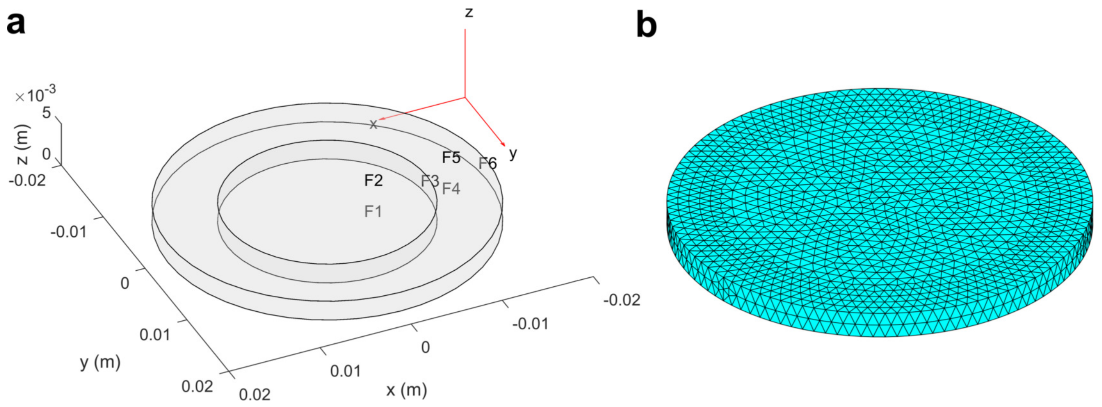


**Figure S3.** Diagram of geometry for heat PDE solver. (**a**) Cylinder geometry representing media volume with a radius of 17.5 mm, an inner radius of 10.95 mm, and a height of 2.269 mm. Faces are labelled. $U_S$ is through F6, $U_W$ is through F5, and $U_B$ is through F1 and F4. (**b**) Mesh geometry showing size and shape of triangular elements.

We choose to simulate using a simple multi-cylindrical geometry where all but one face (the face in contact with the domed lid) is participating in heat transfer. Next we define thermal properties, internal heat source, and boundary conditions.

```
% For a steady state solution, we need only the thermal conductivity
thermalProperties(thermalmodel, 'ThermalConductivity', .606);

% Heat generation condition
q = 1.632E8; % Q(r) above [=] W/m^3
qFunc = @(region,state) q*(region.y.^2+region.x.^2); % r dependency in Cartesian coord
internalHeatSource(thermalmodel, qFunc); % Pass heat generation function to model

% Temperatures
Tinf = 22; % Coil temperature
Tinc = 37;

```

```
% Boundary conditions
thermalmodel.StefanBoltzmannConstant = 5.670373E-8;
thermalBC(thermalmodel, 'Face', 6,...
                        'ConvectionCoefficient', 9.08, ... % U_S [=] W/(m^2 K)
                        'Emissivity', 0.96, ...
                        'AmbientTemperature', Tinf);

thermalBC(thermalmodel, 'Face', 5,...
                        'ConvectionCoefficient', 3.52, ... % U_W
                        'AmbientTemperature', Tinf);

thermalBC(thermalmodel, 'Face', [1, 4],...
                        'ConvectionCoefficient', 12.04, ... % U_B
                        'AmbientTemperature', Tinc);
```

Solving and plotting,

```
result = solve(thermalmodel);
T = result.Temperature;

figure;
pdeplot3D(thermalmodel, 'ColorMapData', T(:,end), ...
                        'FaceAlpha', 0.5);

figure;
pdeplot3D(thermalmodel, 'ColorMapData', T(:,end), ...
                        'FaceAlpha', 1);
view(0, 0) % Bottom view
```

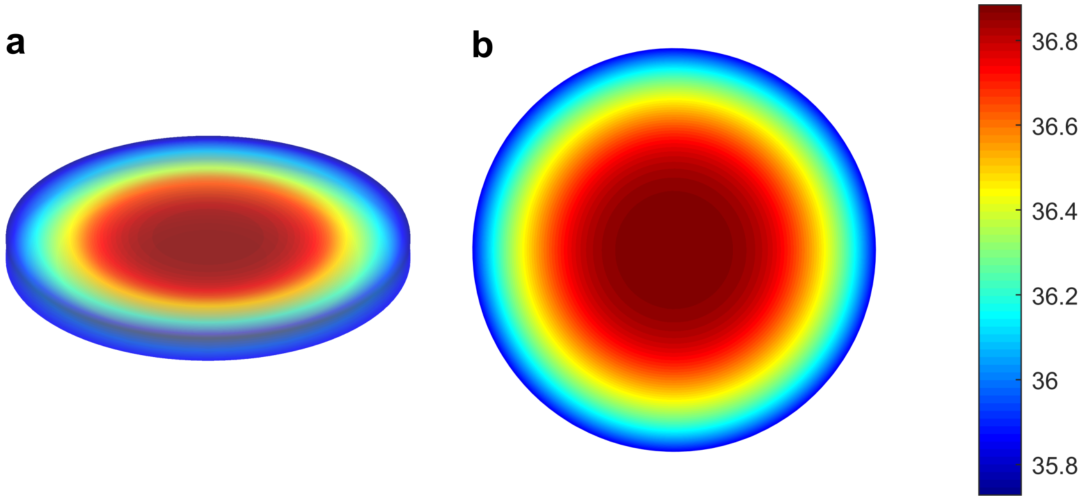


**Figure S4.** Steady state temperature solution using calculated heat transfer coefficients and boundary conditions. (**a**) Steady state temperature profile in whole media volume. (**b**) Bottom profile view.

Results with this set of assumptions predicts decent temperature homogeneity everywhere; temperature variation throughout the dish bottom is within about 1 °C and is, most importantly, centered at the expected 37 °C

(or 0.1 °C cooler – which might be explained by a slight overestimation of $U_W$ or $U_S$ or underestimation of $\dot{q}$). The predicted profile broadly agrees with our temperature measurements in Fig. 4. Similar central and midway temperatures are observed, with notable temperature drop-off at the edge. However, the experimentally measured profile is more homogeneous. A $\sim 0.5\,°\mathrm{C}$ drop-off is observed as compared to the $\sim 1\,°\mathrm{C}$ drop-off in Fig. S4. This increased homogeneity might be explained by mechanical mixing of the dish by vibration of the incubator that is not accounted for here. This mechanical mixing might sufficiently enhance heat transfer within the media to homogenize temperature gradients.

The predicted temperature profile in the absence of active coil cooling is also informative. This situation would be akin to performing the experiment in an incubator without cooling the coil below the set-point of the incubator. The only change in code is:

```
Tinf = 37; % Coil = incubator temperature
```

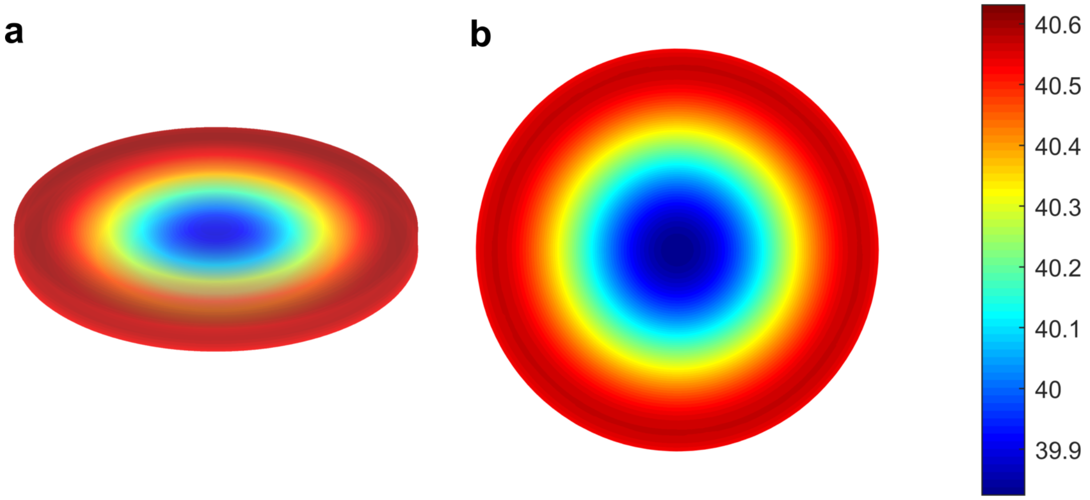


**Figure S5.** Steady state temperature solution using calculated heat transfer coefficients but modified ambient temperature. (**a**) Steady state temperature profile in whole media volume. (**b**) Bottom profile view.

This condition results in temperatures more than 3 °C warmer than the incubator temperature, with a similar radial profile to Fig. S4. This temperature profile would be detrimental to cell growth, and highlights the necessity of careful thermal regulation *beyond* simple incubation.

## Conclusions

We find that temperature homogeneity at steady state is good, and maximal 0.5 – 1 °C differences throughout the dish are expected. We demonstrate that simple incubation is insufficient to maintain temperatures suitable for cell culture. Convective heat transfer contributions are important. Enhancing convective heat transfer by adding fins or baffles to dishes and/or the sleeve might be a worthwhile experimental improvement. Note, permanent incubator and chiller set-points would be insufficient for thermal control, as *the amount of Joule heating changes over the course of the experiment* due to media loss (see Fig. 4a in main text). Media loss changes $L_z$, which we have assumed to be constant in the modeling. Changes in $L_z$ alter the total heat generation. Some form of dynamic controls scheme like the simple, open-loop control used here is necessary.

## 2.5 Internal heat fluxes and Rayleigh–Bénard convection

Temperature gradients were observed in our model. These temperature gradients can lead to directional heat flux within the dish. In some conditions, namely large $z$-axis gradients, these gradients can lead to the formation of convection cells in a process known as Rayleigh–Bénard convection. The rise and fall of water in a boiling kettle is an everyday example of this phenomenon. We must assess whether or not Rayleigh–Bénard convection is present. If it is, it represents a possible experimental confound. We can readily extract the heat fluxes within the dish to get an idea of what the flux directions are, shown below for the temperature profile in Fig. S4.

```
[X,Y,Z] = meshgrid(-R:R/6:R,-R:R/6:R,0:Lz/3:Lz);
[qx,qy,qz] = evaluateHeatFlux(result,X,Y,Z);

qx = reshape(qx,size(X));
qy = reshape(qy,size(Y));
qz = reshape(qz,size(Z));

figure
quiver3(X,Y,Z,qx,qy,qz, 'linewidth',1)
```

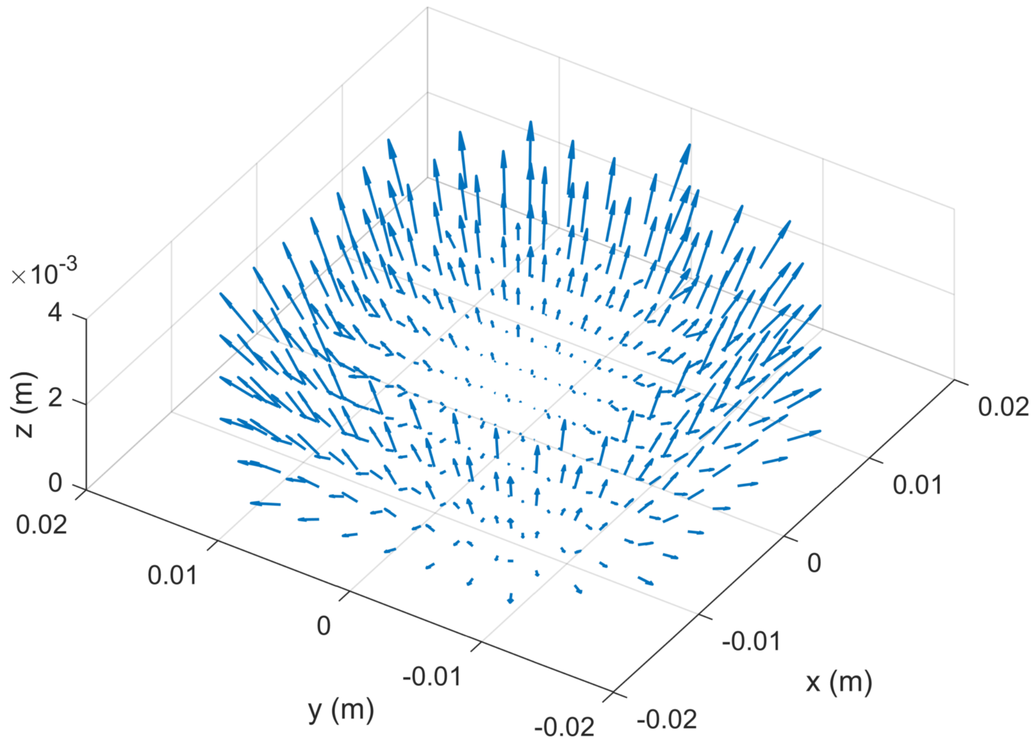


**Figure S6:** Heat flux vectors in the dish. Arrow thickness corresponds to magnitude.

There are some intricacies in the heat flux profile in Fig. S6. Overall, the clearest feature is upwards flux. In the case of upwards flux with a free boundary at the top, i.e., hot surface on the bottom, like a kettle, the

heuristic instability limit for the Rayleigh number is $\mathrm{Ra}_L = 1,100.65$. We can calculate the Rayleigh number from previously determined parameters to find the temperature difference needed to observe instability,

$$\begin{aligned}\mathrm{Ra}_L &= \frac{g\beta\rho c_p}{(\mu/\rho)k}(T_{\mathrm{bottom}} - T_{\mathrm{top}})L^3 \\ &= \frac{(9.81\ \mathrm{m}\cdot\mathrm{s}^{-2})(2.984\times10^{-4}\ \mathrm{K}^{-1})(995.82\ \mathrm{kg}\cdot\mathrm{m}^{-3})(4.18\times10^{3}\ \mathrm{J}\cdot\mathrm{kg}^{-1}\cdot\mathrm{K}^{-1})}{(8.055\times10^{-4}\ \mathrm{N}\cdot\mathrm{s}\cdot\mathrm{m}^{-2}/995.82\ \mathrm{kg}\cdot\mathrm{m}^{-3})(0.624\ \mathrm{W}\cdot\mathrm{m}^{-1}\cdot\mathrm{K}^{-1})} \\ &\quad \times L^3\Delta T \\ &= 2.41\times10^{10}(8.75\times10^{-3}\ \mathrm{m})^3\Delta T \\ &= 16150\Delta T\end{aligned} \tag{24}$$

where the characteristic length is $R/2$. $\Delta T$ would need to exceed 0.07 °C to reach the heuristic instability limit. The top to bottom temperature difference is qualitatively small as shown by comparing the top profiles and bottom profiles in Figs. S4a and b or Figs. S5a and b. Looking at interpolated temperature data, differences from top to bottom range from effectively $0$ ($\ll 0.1$ °C) towards the middle to $\sim 0.1$ °C nearer to the edge. Thus, minor Rayleigh–Bénard effects might appear according to the modeling, but only locally at the dish edge – no larger convection cells are expected. We also infer that if we incorporate mixing and enhanced thermal conductivity, the instability limit would not be reached even at the edge. Indeed, no convective behavior was observed experimentally. Rayleigh–Bénard effects are not anticipated to contribute to observed treatment results.

# 3 Image processing and threshold selection

Details of the lower intensity threshold selection were not included in the main body of the paper. We present those details here along with intensity histograms for an example region (189 $\times$ 189) going through the thresholding process described in Figs. 2a – 2d. MATLAB code demonstrating the operations is provided. Code for the process in Figs. 2e – 2h is functionally identical and can be extrapolated from the code provided here.

## 3.1 Contrast enhancement

After reading in the image (which may require the freely available Bio-Formats toolbox), the first processing step is contrast enhancement via morphological transforms followed by Wiener filtering with a 3 $\times$ 3 matrix.

```
se = strel('disk', 3);      % Structuring element
img = imsubtract(imadd(img, imtophat(img, se)),...
                            imbothat(img ,se));
img(img > 1) = 1;           % Floor intensities exceeding 1
img = wiener2(img, [3 3]); % Wiener filtering
```

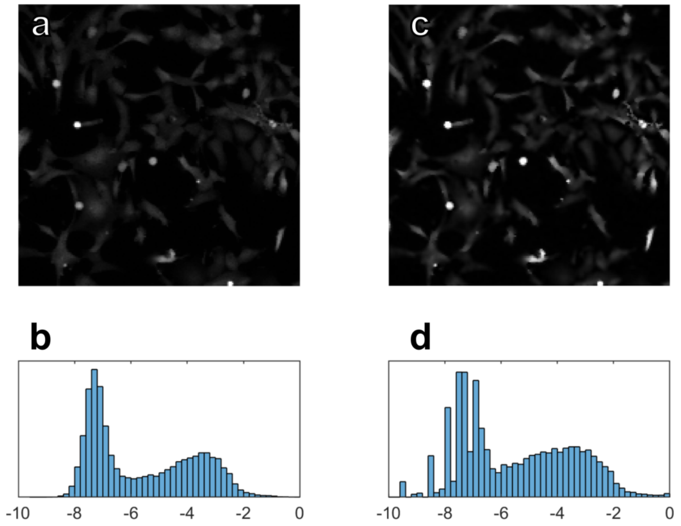


**Figure S7:** First image processing step of morphological contrast enhancement and Wiener filter denoising. (**a**) Raw image, (**b**) corresponding log scale intensity histogram. (**c**) Contrast enhanced and denoised image and (**d**) intensity histogram.

The contrast enhancement step has the effect of broadening the intensity histogram while retaining the same overall shape. Very few px become saturated (0 on the log scale) as shown in Fig. S7.

## 3.2 Threshold selection

Next, we determine the upper threshold using Otsu's method,

```
th = multithresh(img2, 2); % Otsu's method with two thresholds
hi_th = th(2);             % Upper threshold
```

Consider that we want the lower threshold to trace the edges of the dimmer population of cells. We can pick a threshold that will do this in a few steps. First, we perform standard deviation filtering (3×3 ones matrix) and threshold the filtered image into 3 populations. Intuitively, the smallest deviation population will be background or cell interiors, the middle population will be the edges of dim cells, and the largest population will be the edges of bright cells. We can take the middle population and use it as a mask on our contrast enhanced image to extract only the edges of dim cells. Then, we can pick an intensity threshold that will keep 75% of the px identified by standard deviation filter as belonging to the edges of dim cells. The threshold will therefore "trace" the edges of the dimmer population of cells. This procedure is outlined in the code and Fig. S8 below.

```
img_std = stdfilt(img2, ones(3));          % Standard deviation filtered image
std_th = multithresh(img_std, 2);          % Threshold the filtered image into 3 populations
img_std_th = imquantize(img_std, std_th); % Quantize the image: 1, 2, 3 - mapped to ...
    black, white, red below

img_std_th(img_std_th ≠ 2) = 0   % Keep only the middle population
img_masked = img(img_std_th == 2) % Mask the contrast enhanced image

[f, x] = ecdf(img_masked);
cutoff = 0.25;
lo_th = x(sum(f < cutoff)); % Pick an intensity that keeps 25\% of masked px using an ...
    empirical cumulative distribution function
```

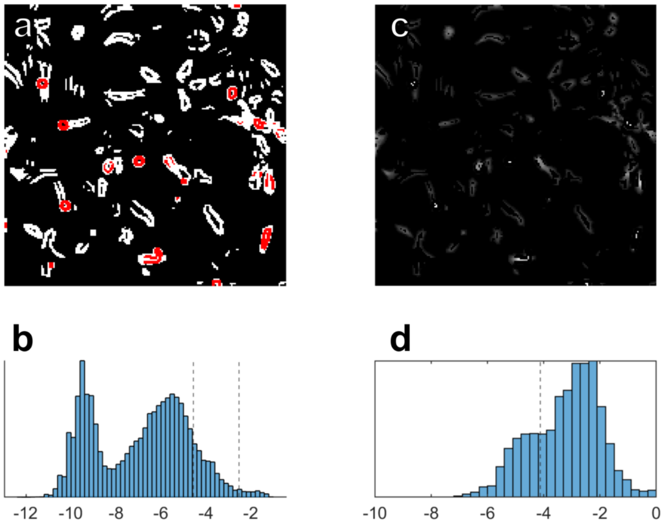


**Figure S8:** Lower threshold selection process. (**a**) Standard deviation filtered and quantized image. The three populations correspond roughly to background/centers (black), edges of dim cells (white), and edges of bright cells (red). (**b**) Intensity histogram of filtered image. Thresholds identified and used to generate quantized image above are marked with dashed lines. (**c**) Masked contrast enhanced image, using the white px in the left image as the mask. (**d**) Intensity histogram of masked image with selected low threshold marked. Low threshold removes the bottom 25% of the histogram.

With the low and high thresholds chosen, the contrast enhanced image is quantized,

```
img_th = imquantize(img, [lo_th hi_th]);
```

### 3.3 Classification error correction

As discussed in the main text and the methods, classification errors need to be corrected. The edges of bright regions are sometimes incorrectly classified as dim px due to intensity drop-off (like a "halo" of dim px) and small pockets of bright px ("spots") appear within dim cells. Both types of errors can be corrected by looking at all contiguous bright regions, determining the type of error, and addressing it. We first extract a binary image of only the px classified as bright and then find all contiguous regions, their area, and their list of px indices.

```
img_bright_bw = (img == 3) % Binary/black-white image of bright px
regions = regionprops(img_bright_bw, 'Area', 'pxList');
```

We then iterate through all regions and correct the two types of errors. If a region is below a certain size cutoff (8 px) *and* most of the surrounding px (> 60%) in the thresholded image are dim, then the bright px are converted to dim px. If a region is above the size cutoff, then the dim px in its perimeter are turned to bright px (background px are left alone) in a flood fill. Two passes of these corrections were performed.

```
for i = 1:length(regions) % Note: 1 = bg, 2 = dim, 3 = bright

    region = regions(i);

    ind = sub2ind(size(img),...
              region.pixelList(:,2),...
              region.pixelList(:,1)); % Get corresponding indices of region in the ...
                  contrast enhanced image

    perim_ind = getPerim(region.pixelList, size(img, 1), size(img, 2)); % Helper ...
        function gets indices of perimeter

    if region.Area < size_cutoff % Below size cutoff of 8 px
        perim_live = sum(img(perim_ind) == 2)/length(perim_ind); % Percentage of dim px ...
            in perimeter

        if perim_live > bord_cutoff % Percentage cutoff of 0.6
            img2(ind) = 2; % Convert bright region to dim
        else
            continue
        end
    else
    img2(perim_ind(img(perim_ind) == 2)) = 3; % If above size cutoff, then fill ...
        perimeter with bright px
end
```

In Fig. S9 below, we compare naïve Otsu's thresholding to our in-house pipeline with lower threshold adjustment and additional classification error corrections. This pipeline was used on all 36 control dishes (P2, P4, P5), taking a large central section. Lower and upper thresholds were determined for each control dish. The distribution of identified thresholds is shown in Fig. S10. From these distributions, the *average* threshold values (low = 0.0635, high = 0.3727) were used on *all* dishes for consistency across analyses of both control and treated dishes.

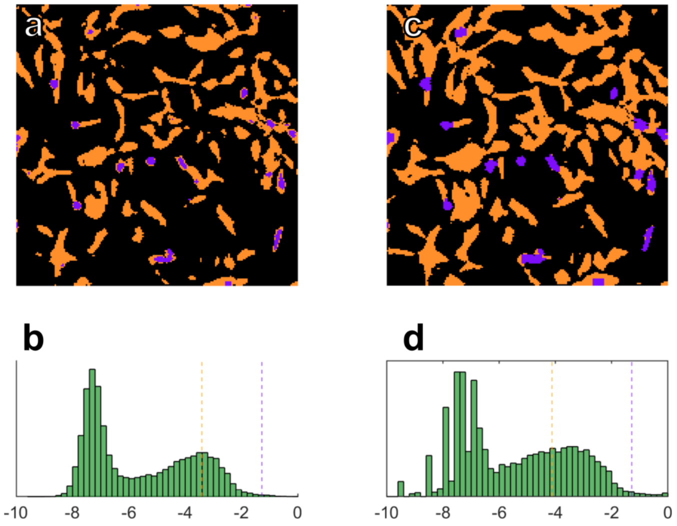


**Figure S9:** Final quantization and error correction process. (**a**) Naïve Otsu's thresholding after contrast enhancement. (**b**) Intensity histogram with marked lower and upper thresholds. (**c**) In-house pipeline with lower threshold adjustment and error corrections described. (**d**) Intensity histogram with lower and upper thresholds marked. Lower = orange, upper = violet.

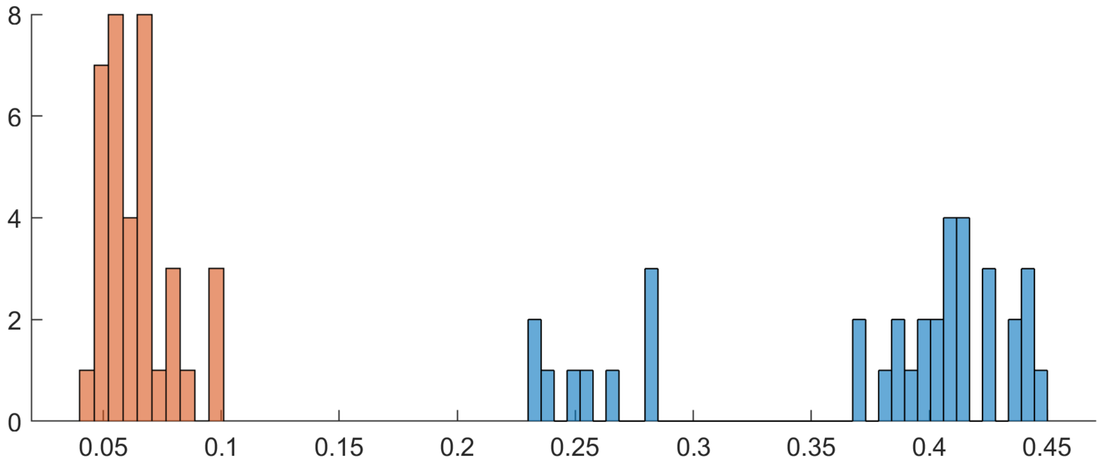


**Figure S10:** Distributions of selected thresholds. Orange = low, blue = high.

# References


[1] J. Welty, C. E. Wicks, G. L. Rorrer, R. E. Wilson, Fundamentals of momentum, heat, and mass transfer, Wiley, Hoboken, NJ, 2015.

[2] F. A. Schwertz, J. E. Brow, Diffusivity of Water Vapor in Some Common Gases, The Journal of Chemical

Physics 19 (5) (1951) 640–646. doi:10.1063/1.1748306.

[3] V. Teske, E. Vogel, E. Bich, Viscosity Measurements on Water Vapor and Their Evaluation, Journal of Chemical & Engineering Data 50 (6) (2005) 2082–2087. doi:10.1021/je050288d.

[4] S. Chapman, T. G. Cowling, D. Burnett, The Mathematical Theory of Non-uniform Gases: An Account of the Kinetic Theory of Viscosity, Thermal Conduction and Diffusion in Gases, Cambridge University Press, 1990.

[5] W. M. Haynes, CRC Handbook of Chemistry and Physics, 92nd Edition, CRC Press, 2011.

[6] F. Herning, L. Zipperer, Calculation of the viscosity of technical gas mixtures from the viscosity of the individual gases, Gas u. Wasserfach 79 (1936) 69.

[7] C. R. Wilke, A Viscosity Equation for Gas Mixtures, The Journal of Chemical Physics 18 (4) (1950) 517–519. doi:10.1063/1.1747673.

[8] R. B. Bird, W. E. Stewart, E. N. Lightfoot, Transport Phenomena, Revised 2nd Edition, John Wiley & Sons, Inc., 2006.

[9] C. A. Harper, Modern Plastics Handbook, McGraw-Hill Professional, 2000.

[10] S. W. Churchill, H. H. S. Chu, Correlating equations for laminar and turbulent free convection from a horizontal cylinder, International Journal of Heat and Mass Transfer 18 (9) (1975) 1049 – 1053. doi:https://doi.org/10.1016/0017-9310(75)90222-7.

[11] W. H. McAdams, Heat Transmission, Krieger Pub Co, 1985.

[12] M.-T. Chen, C. Jiang, P. T. Vernier, Y.-H. Wu, M. A. Gundersen, Two-dimensional nanosecond electric field mapping based on cell electropermeabilization, PMC Biophysics 2 (2009) 9. doi:10.1186/1757-5036-2-9.

[13] W. Arnold, G. Fuhr, Increasing the permittivity and conductivity of cellular electromanipulation media, in: Proceedings of 1994 IEEE Industry Applications Society Annual Meeting, Vol. 2, 1994, pp. 1470–1476 vol.2. doi:10.1109/IAS.1994.377619.

[14] N. Mittal, A. Rosenthal, J. Voldman, nDEP microwells for single-cell patterning in physiological media, Lab on a Chip 7 (9) (2007) 1146. doi:10.1039/b706342c.
